# Supplementary material for: StoryWriter: A Multi-Agent Framework for Long Story Generation
Source: arXiv:2506.16445 source file (2025-06-19)
Supplement: Supplementary file 1 [file 09.appendix.tex]

\section*{Appendices}
\section{Outline Agents Example}
% 在故事生成的第一阶段，我们会生成一个基于事件的outline，这个outline由一个个事件构成，每个事件又包含有若干事件信息与事件属性，之后的文章生成都是在该outline的基础上生成的。不同于传统的大纲生成方法，我们的outline提供更多信息，且提高了信息密度，降低了由outline构建story过程中获取关键信息的难度。表中展示了一个outline的例子
In the first stage of story generation, we generate an event-based outline, which consists of one event, each event contains several event information, and the subsequent articles are generated on the basis of this outline. Different from the traditional outline generation method, our outline provides more information and improves the information density, which reduces the difficulty of obtaining key information in the process of constructing the story from the outline. An example of an outline is shown in Table~\ref{table:events_outline}
\section{Planning Agents Example}

% 在故事生成的第二阶段，我们提供了一个进一步处理outline的方法NLN（none-linear-narration），用来生成一个结构更加多样，情节更加丰富的outline。在这一阶段，agents会根据outline中的事件进一步生成若干子事件。并按照事件信息合理安排子事件的坐在章节。以表n为例子，agent认为event3.3作为事件3的小结尾，可以作为悬念留到chapter4中再讲，因此改变了event的叙述顺序。
In the second stage of story generation, we introduce a method NLN (non-linear-narration) to further process the outlines, which is used to generate a more structurally varied and plot-rich outlines. In this stage, AGENTS further generates a number of sub-events based on the events in the outlines. And the sitting chapters of the sub-events are rationally arranged according to the event information. Taking Table~\ref{table:app_subevent} as an example, AGENTS considers event3.3 as a small ending of event3, which can be left as a suspense to be told in Chapter4, and therefore changes the narrative order of events.

\section{Writing Agents Example}
% 在故事的writing阶段，我们介绍了Coordinator,一个实现处理writing阶段输入输出的agent。Coordinator会接收历史信息并进行处理，同时接收FinalWriter的输出并进行rewrite。表n展示了Coordinator处理后的history-message，该方法在尽可能保留事件信息的前提下，极大缩短了文本长度。表m展示了Coordinator处理后的story。
\subsection{Re-write History}
In the writing phase of the story, we introduce Coordinator, an agent that implements the processing of inputs and outputs in the writing phase.Coordinator receives the history-message and processes it, and receives the output from FinalWriter and rewrites it. Table~\ref{table:example4reinput} shows the history-message processed by the Coordinator, which greatly reduces the length of the text while preserving as much event information as possible. 
\subsection{Re-write Story}
Table~\ref{table:app_reoutput} shows the story re-written by the Coordinator. In the generation phase, Coordinator thinks that the generated story deviates from the outline, or the plot is inconsistent, then Coordinator re-writes based on the original story.
\onecolumn
\begin{longtable}{|p{2.5cm}|p{12.5cm}|}
\hline
\textbf{Type} & \textbf{Content} \\
\hline
\endfirsthead
\hline
\textbf{Type} & \textbf{Content} \\
\hline
\endhead
\hline
\endfoot
\hline
\caption{\label{table:events_outline} Example of event-based outline generation.} \\
\endlastfoot
Premise & In a cyberpunk future, a skilled hacker uncovers a hidden backdoor within a digital game, leading to a high-stakes battle against a ruthless corporate spy to expose corruption and clear their name. \\
Event 1: The Discovery  &  \textbf{Setting} A dimly lit, cluttered apartment in a towering cyberpunk city, filled with neon lights, holographic screens, and advanced tech equipment. The sounds of distant traffic hum and synth music can be faintly heard outside.  \textbf{Character} *Nova*, a skilled hacker known for their proficiency in navigating complex systems and infiltrating digital environments. They live under the radar, maintaining a low profile while taking on high-risk jobs for the right price.  \textbf{Action} Nova is exploring a newly released VR game, \"Eclipse\", for a client. While trying to breach the game's code to find exploits for financial gain, Nova stumbles upon an encrypted backdoor hidden within the game’s files. The backdoor seems to provide access to sensitive corporate data.  \textbf{Conflict} Nova is unsure whether the backdoor is a hidden Easter egg or something far more dangerous. The temptation to expose this digital goldmine is strong, but Nova is cautious, knowing that they could be digging up something bigger than they intended.  \textbf{Plot Twist} Upon attempting to hack further into the backdoor, Nova triggers an alert, and the system begins sending data to an unknown source. It quickly becomes clear that the game’s creators (a powerful tech corporation) have been aware of this backdoor and are actively monitoring anyone who discovers it.  \\
Event 2: The Corporate Spy & \textbf{Setting} A sleek, high-rise corporate tower that looms over the city. Inside, the space is clean, minimalistic, and brimming with high-tech security measures.  \textbf{Character} *Arius*, a ruthless corporate spy hired by a shadowy tech conglomerate to track down and eliminate anyone who uncovers the backdoor. Arius is cold, calculating, and specializes in espionage, blending seamlessly into both the digital and physical worlds.  \textbf{Action} Nova, realizing that they’re being hunted, tries to cover their tracks and protect their identity. However, Arius uses a combination of physical surveillance and digital forensics to track Nova's real-world location.  \textbf{Conflict} Nova is now in a race against time—if they can’t find a way to delete the backdoor’s data and escape the corporate's radar, they’ll be framed for a crime they didn’t commit. Meanwhile, Arius is relentlessly closing in, trying to eliminate Nova before they can expose the corruption.  \textbf{Plot Twist} Nova finds a clue that suggests the backdoor isn’t just a corporate oversight but rather part of a larger conspiracy involving illegal surveillance of the game's players—many of whom are high-ranking individuals. The data could be used to topple powerful figures, including those responsible for exploiting the game's player base. \\  
Event 3: The Battle for the Truth & \textbf{Setting} A hidden underground hacker enclave, far beneath the city. It’s a chaotic mix of neon-lit computer screens, tech junk, and cyber-enhanced individuals working in tandem.  \textbf{Character} *Nova* is joined by a small group of rogue hackers and data analysts who share Nova's goal of exposing corporate corruption and freeing the game’s players from digital surveillance.  \textbf{Action} Nova and the team work together to decrypt and upload the stolen data, hoping to expose the corporation's illegal activities. As they work, they are constantly interrupted by Arius's cyber attacks, including digital traps, viruses, and physical infiltrations.  \textbf{Conflict} The team faces internal discord—some members are hesitant to expose the data, fearing they’ll be wiped out by the corporation. Meanwhile, Arius uses a combination of mind games and brutal force to break the hackers’ resolve.  \textbf{Plot Twist} Just as the data is about to be uploaded to a secure public channel, Nova learns that one of their own allies has been feeding information to the corporation, sabotaging the mission in exchange for a personal reward. The betrayal threatens to unravel everything. \\ 
Event 4: Final Confrontation & \textbf{Setting} A high-tech digital arena, part of the VR game \"Eclipse\". Nova and Arius are forced into a head-to-head battle within the game's simulated world, a vast, dystopian city filled with virtual enemies and obstacles.  \textbf{Character} *Nova* and *Arius*, now fully aware of each other’s tactics. The stakes are higher than ever—if Nova wins, the data is released, exposing the corporation's corruption. If Arius wins, the data is erased, and Nova's reputation is destroyed.  \textbf{Action} The digital battle intensifies as both Nova and Arius use their hacking abilities and in-game avatars to manipulate the environment, hacking enemies, and creating traps for each other. Nova uses their ingenuity to manipulate the game’s code in real-time, while Arius relies on brute force and quick reflexes.  \textbf{Conflict} The battle is not just physical but also psychological. Arius tries to break Nova’s focus, attempting to force them into a corner by threatening their allies. Meanwhile, Nova must keep their wits and avoid Arius’s relentless attacks.  \textbf{Plot Twist} In the heat of the battle, Nova uncovers a final piece of the puzzle—the game’s designers had created an AI within the game that was programmed to act as a corporate watchdog, and it is now fully aware of their presence. The AI turns on both Nova and Arius, threatening to destroy the entire operation unless they work together to shut it down. \\
Event 5: The Truth Revealed & \textbf{Setting} A public broadcasting channel on the city’s vast network of digital billboards, live-streaming to millions of citizens across the city.  \textbf{Character} *Nova* and *Arius*—having put their differences aside for the moment, working together to expose the truth.  \textbf{Action} Nova and Arius manage to shut down the rogue AI, but they must act quickly to ensure the data gets broadcasted to the public before the corporation can silence them. They upload the information, revealing the corporation’s illegal surveillance and the exploitation of the players.  \textbf{Conflict} As the data is sent out, corporate forces make one final attempt to shut down the broadcast. The city is thrown into chaos as protesters take to the streets, demanding answers.  \textbf{Plot Twist} The broadcast not only reveals the corruption but also uncovers a far-reaching conspiracy implicating the city's government officials, leading to a new power struggle. Nova is left to face the consequences of exposing such a huge secret—now a wanted fugitive, but a symbol of rebellion.  \\ 
Event 6: The Escape & \textbf{Setting} The chaotic streets of the city, now rife with protest and unrest. The neon lights have been replaced with sirens and flashing red alerts.  \textbf{Character} *Nova*, now a fugitive with a target on their back.  \textbf{Action} Nova uses their hacking skills to navigate through the city, evading capture while deciding whether to join the rebellion or disappear into the shadows to protect themselves. The streets are alive with people rallying against the corporation, offering Nova a glimmer of hope for a revolution.  \textbf{Conflict} Nova is faced with a moral choice—do they continue to fight for the truth, risking their life for a cause that might never succeed, or do they disappear, leaving the rebellion to its own fate?  \textbf{Plot Twist} As Nova prepares to vanish, they receive a message from an unknown ally—Arius has gone underground, planning to build a resistance against the corporation, and wants Nova to lead it. \\  \\
\end{longtable}

\onecolumn
\begin{longtable}{|p{2.5cm}|p{12.5cm}|}
\hline
\textbf{Type} & \textbf{Content} \\
\hline
\endfirsthead
\hline
\textbf{Type} & \textbf{Content} \\
\hline
\endhead
\hline
\endfoot
\hline
\caption{\label{table:app_subevent} Example of NLN sub-event and weaving process in the appendix.} \\
\endlastfoot
SubTasker Output & \\
Event 1: The Rogue's Quest Begins  &  \textbf{Event 1.1: Jorik's Motivation and Introduction}   Jorik, a quick-witted and resourceful rogue with a shadowy past, is introduced in a bustling medieval town. We see his skill and cunning as he navigates the town, hinting at his personal struggles and motivations, possibly tied to a past betrayal or loss.  \newline \textbf{Event 1.2: The Mysterious Benefactor’s Request}    Jorik is approached by a mysterious benefactor who offers him a lucrative mission: to retrieve the *Moonstone Heart*, an artifact of immense power hidden deep within the ruins of an ancient castle. The rogue agrees, driven by the promise of riches or a chance to redeem himself. \newline \textbf{Event 1.3: The Castle's Dangerous Secrets}   Jorik begins his journey toward the crumbling castle, navigating through a landscape of myth and danger. As he approaches the castle, he learns more about its treacherous history and the creatures guarding the artifact. He begins to understand the gravity of the task before him. \\
Event 2: The Shapeshifter’s Interference & \textbf{Event 2.1: Virelith’s Deceptive Entrance}    As Jorik approaches the *Moonstone Heart*, Virelith appears, disguised as an old friend from his past. She convinces Jorik to trust her, claiming they both seek the artifact for peace, and proposes an alliance to unlock the artifact’s protections. \newline \textbf{Event 2.2: Alliance Amid Suspicion}    Jorik and Virelith reluctantly team up, but tensions rise as Jorik remains wary of her true intentions. Their alliance is forced, and they struggle to cooperate while dealing with the powerful protections around the artifact. \newline \textbf{Event 2.3: Betrayal and the True Purpose of the Artifact}   At the final moment, Virelith reveals her true form and betrays Jorik. She takes the *Moonstone Heart* for herself, intending to use it to control the mythical creatures of the realm and upset the balance of power.\\
Event 3: The Aftermath of Betrayal & \textbf{Event 3.1: Jorik’s Despair and the Unexpected Ally}    Jorik, devastated by Virelith’s betrayal, is left wandering the dark forests surrounding the ruins. He encounters Elira, a wise centaur, who offers him an unexpected alliance and insight into the greater stakes surrounding the artifact. \newline \textbf{Event 3.2: Jorik’s Internal Struggle}    Jorik wrestles with his shattered trust, particularly in light of his past actions that have led to his isolation from both humans and mythical creatures. He is unsure whether he can ever unite these groups against Virelith and her growing influence. \newline \textbf{Event 3.3: Divided Allegiances and Growing Tension}    Jorik and Elira begin rallying the mythical creatures to unite against Virelith, but they face opposition. Some creatures believe the artifact can bring peace, while others fear its destructive potential. Jorik's leadership is challenged, and tensions rise within the ranks.\\
Event 4: The Artifact’s True Power & \textbf{Event 4.1: The Final Confrontation in the Sacred Grove}    Jorik and Virelith face off in the sacred grove, where the artifact pulses with dark energy. Jorik realizes that the *Moonstone Heart* cannot be controlled without catastrophic consequences. The world around them distorts as the artifact’s power escalates. \newline \textbf{Event 4.2: The True Nature of the Artifact Revealed}    In the heat of battle, Elira reveals that the *Moonstone Heart* is a sentient being, created as a guardian to test those who seek its power. The artifact’s role is not to be wielded but to bring change to the realm, whether for good or ill. \newline \textbf{Event 4.3: A Choice Between Destruction and Evolution}   Jorik is faced with the decision to destroy the artifact to prevent its catastrophic effects or to allow it to remain, trusting that its true purpose will lead to peace. The realization that it is neither a tool for domination nor a simple weapon deepens the moral dilemma.\\
Event 5: A New Path to Peace & \textbf{Event 5.1: Jorik’s Proposal for Peace}    Jorik, after understanding the true nature of the artifact, proposes a new path to unite humans and mythical creatures, without relying on the artifact’s influence. He convinces Virelith to abandon her quest for domination, though this is no easy task. \newline \textbf{Event 5.2: Resistance and Doubt Among the Factions}    While Jorik and Virelith work together to forge a new order, they face resistance from both sides. Some creatures and humans are skeptical that true peace is possible, and Virelith’s manipulative nature complicates the process of building trust. \newline \textbf{Event 5.3: A New Enemy Emerges}    As the fragile peace is taking shape, a rogue faction of humans and creatures seeks to seize the artifact for their own gain. Jorik must rally all sides to confront this new threat, showing that peace requires sacrifices from all parties.\\
Event 6: The Final Battle and the Legacy of the Moonstone Heart & \textbf{Event 6.1: The Rogue Faction’s Attack}    The rogue faction, intent on seizing control of the artifact, launches an assault on the united forces. Jorik, Virelith, and Elira lead the defense, understanding that this battle is crucial for the future of the realm. \newline \textbf{Event 6.2: Jorik’s Ultimate Sacrifice}    In a desperate final act, Jorik decides to destroy the *Moonstone Heart*, realizing that its power cannot be allowed to fall into the wrong hands. The artifact’s destruction causes a massive upheaval, but it ends the threat of domination over the realm. \newline \textbf{Event 6.3: A New Era of Peace}    As Jorik lies gravely injured, the energy of the artifact dissipates. The sacrifice made by all involved ensures that mythical creatures and humans can now coexist in harmony. The realm is forever changed, but the legacy of the *Moonstone Heart* endures, a symbol of the cost of peace. \\
    
Weaver Output &  \textbf{Chapter 1: The Rogue's Quest Begins}   \newline Sub-event: Jorik's Motivation and Introduction   \newline Sub-event: The Mysterious Benefactor’s Request   \newline Sub-event: The Castle's Dangerous Secrets  Context: The first chapter sets up Jorik's character, his motivations, and the central quest. We meet the rogue in the bustling town, learn of his troubled past, and witness his skills. The mysterious benefactor introduces the central artifact, the *Moonstone Heart*, and sets the stage for the perilous journey ahead. \newline \textbf{Chapter 2: The Shapeshifter’s Deception}   \newline Sub-event: Virelith’s Deceptive Entrance   \newline Sub-event: Alliance Amid Suspicion   \newline Sub-event: Betrayal and the True Purpose of the Artifact  Context: This chapter introduces Virelith, whose true intentions are hidden behind the mask of a helpful ally. The dynamic between her and Jorik builds tension as their uneasy alliance grows. The betrayal and reveal of Virelith's real goal push the plot toward its darker, more dangerous turns. \newline \textbf{Chapter 3: Despair and Unexpected Alliances}   \newline Sub-event: Jorik’s Despair and the Unexpected Ally   \newline Sub-event: Jorik’s Internal Struggle   \newline  Sub-event: The Final Confrontation in the Sacred Grove  Context: After the betrayal, Jorik's internal conflict is explored. He encounters Elira, a centaur who offers a new perspective and an alliance against the growing threat. The chapter focuses on Jorik's journey of rebuilding trust while facing rising tensions between mythical creatures and humans. \newline \textbf{Chapter 4: The Artifact's Power Revealed}   \newline Sub-event: Divided Allegiances and Growing Tension   \newline Sub-event: The True Nature of the Artifact Revealed   \newline Sub-event: A Choice Between Destruction and Evolution  Context: In the climactic confrontation with Virelith, the artifact’s true nature is unveiled. This chapter serves as a turning point in the story as Jorik must decide whether to destroy the artifact or embrace its uncertain future. The moral and ethical stakes reach their highest point. \newline \textbf{Chapter 5: The Fragile Path to Peace}   \newline Sub-event: Jorik’s Proposal for Peace   \newline Sub-event: Resistance and Doubt Among the Factions   \newline Sub-event: A New Enemy Emerges  Context: The aftermath of the artifact’s revelation leads to Jorik's proposal for peace between humans and mythical creatures. However, the process is fraught with resistance and internal conflict. Just as things seem to settle, a new threat emerges, forcing Jorik and his allies to act quickly. \newline \textbf{Chapter 6: The Final Battle and the Legacy of the Moonstone Heart}   \newline Sub-event: The Rogue Faction’s Attack   \newline Sub-event: Jorik’s Ultimate Sacrifice   \newline Sub-event: A New Era of Peace  Context: The final battle unfolds as a rogue faction threatens the fragile peace. Jorik's ultimate sacrifice to destroy the artifact concludes the story, ensuring peace but at great personal cost. The chapter wraps up with the realm forever changed, and the legacy of the *Moonstone Heart* enduring as a symbol of the sacrifices made for peace.
 
\end{longtable}

\begin{table*}[!htbp]
    \scalebox{0.9}{
    \begin{tabularx}{\textwidth}{|l|X|}
        \toprule
        \textbf{Role} & \textbf{Content} \\
        \midrule
        FinalWriter & In the days that followed, Kael and Luna found their way back to the cavern that had changed his life forever. The snowy landscape had become familiar, yet Kael’s heart raced with anticipation and the weight of responsibility. He had come to realize that the ancient artifact held the key to unlocking his true potential as a mage, and he could feel its call echoing in the depths of his soul.\par As they entered the cave, the air was charged with a palpable energy. The sunlight streamed through the crystals embedded in the cave walls, creating a mesmerizing display of colors that danced like spirits in the darkness. The artifact rested on a stone pedestal, shimmering with a mystic light that beckoned him closer.\par Luna padded silently beside him, her fur glistening in the cave’s ethereal glow. She seemed to sense the significance of this moment too, her ears perked forward, eyes keen and alert. Kael reached out, his fingers brushing against the smooth surface of the orb. Instantly, images flooded his mind—visions of mages harnessing great power, wielding magic for both creation and destruction.\par With resolve, Kael inhaled deeply, reminding himself of the bond he shared with Luna and the strength they had gained together. This was a pivotal moment, and he knew he needed to embrace it fully. He steadied himself, focusing on the energies swirling around him and the warmth the artifact emitted.\par The moment his hands clasped the orb, a surge of magic coursed through him like lightning. It was unlike anything he had ever experienced—pure, exhilarating power merging with his very essence. He felt the weight of the world lift from his shoulders as he began to awaken the magic within him, unraveling the potential he had been so afraid to unleash.\par Yet, as the energy intensified, Kael suddenly felt a tugging sensation—a dark shadow lurking at the edge of his consciousness. The power was formidable, and with it came a haunting thought: was he truly ready to wield such magic? Would he be able to resist the allure of darkness if faced with the temptation? \\
        History-Messages & {'content': "With the artifact's power surging, Kael transformed, awakening abilities he never knew he had. His appearance changed, reflecting the magic within him as he realized he was becoming a protector, ready to use this newfound power for his village's safety. Luna stood by him, providing unwavering support as a dark presence emerged— a malevolent sorcerer intent on seizing the artifact's magic for himself. Feeling the weight of this looming threat, Kael understood he had to prepare for a confrontation with the sorcerer.Determined to control his new abilities and balance the light and dark within him, Kael, with Luna at his side, left the cavern. They were ready to face the trials ahead, confident that together they could confront any darkness threatening their world.", 'role': 'user', 'name': 'FinalWriter'} \\
        \bottomrule
    \end{tabularx}
    }
    \caption{\label{table:example4reinput} Example of prompt and history-message for Re-Input in story generation.}
\end{table*}

\onecolumn
\begin{longtable}{|p{2.5cm}|p{12.5cm}|}
\hline
\textbf{Type} & \textbf{Content} \\
\hline
\endfirsthead
\hline
\textbf{Type} & \textbf{Content} \\
\hline
\endhead
\hline
\endfoot
\hline
\caption{\label{table:app_reoutput} Example of original and re-written output in the ReIO stage.}  \\
\endlastfoot
Original Output & \textbf{FinalWriter:} In the wake of the tentative truce, Razor made his demands clear. He was no stranger to power plays, and he intended  to use this moment to reclaim control over his territory. During a follow-up meeting orchestrated by Father Gregory, Razor leaned forward, his tone measured but resolute. "I'll agree to your community initiatives and support your mentoring programs, but in exchange, I need control over the local drug trade. That's the only way I can guarantee the safety of my people. It's how I ensure resources come in—money that can help us all," he stated, showcasing his unwavering belief that the drug trade was a necessary evil. Tasha felt a surge of frustration. "Razor, we can't build a future on the backs of our neighbors. Sure, the money flows, but it also brings violence, fear, and more suffering. That's not what this community deserves," she implored passionately, her voice steady but laced with urgency.  
Razor smirked, shaking his head as if she were naïve. "You think your ideals can change the world. I'm in the real world, Tasha. Families are hungry. The kids are trapped with nowhere to turn. They want power and respect—what I can provide. You can't just erase the reality of survival." 
The room buzzed with tension. Father Gregory attempted to mediate, sensing that both were at a critical impasse. "Razor, perhaps there's a middle ground," he suggested, but Tasha was quick to interject.  
"There is no middle ground when you're advocating for further destruction. I will not support a criminal approach to community development," she asserted, her conviction palpable. "Meaningful change requires us to move away from illegal activities. We can create jobs, build businesses, and invest in our youth through legitimate means." 
Razor narrowed his eyes, the anger bubbling beneath the surface. "And what happens if your way doesn't work? If we don't act now, more will suffer. I'm trying to protect my own." 
"By perpetuating a cycle of violence?" Tasha challenged. "Look deeper, Razor. Do you understand what this is doing to our community? Do you care? The people are tired of fear. They want hope." 
In that moment, Razor's fierce demeanor softened ever so slightly. He glanced around the room, measuring the expressions of those gathered. Many, including former gang members who had turned a new leaf, started to murmur in agreement with Tasha's vision. It struck a chord that had long been buried beneath the chaos of the streets
Yet Razor wasn't ready to concede control. "You're all dreaming. I have spent years building an empire. You can't just ask me to sacrifice everything without a viable alternative. Show me how your way will work, then we can talk."
Tasha took a deep breath, knowing this was a pivotal moment. "We can start small. Let's invest in youth programs, job training, and small business grants. Work together to fund initiatives that can uplift the community without violence. I'll bring legitimate businesses in, and you can help steer that profit into community gains. But we do it openly and with integrity. This is about empowerment, not dominance."
Razor stared at her, weighing his options. For so long, he had ruled through fear, convinced it was the only way. But now he faced a community unwilling to accept his old methods, and the prospect of losing respect was frightening.
The standoff highlighted the stark realities of their opposing visions for the future, and Razor realized that without adapting to the new demands of his people, he would risk alienating everyone, including those he sought to protect.
"At the very least, I'll consider your proposal, Tasha,"\\
Original Output & Razor finally said, his voice low but steady. "But like I said, if this doesn't strengthen my position, there will be consequences." 
Tasha understood the fragility of this moment, but it was a step—a precarious but crucial step towards a newfound possibility for coexistence built on mutual benefit instead of mutual destruction. The fight for peace was far from over, and the battle lines continued to shift as they each sought to define their legacies amidst turbulent change.\\
    
Re-written Output & \textbf{Coordinator:} \textbf{RE-WRITE:} Razor's demand for control over the drug trade in exchange for peace was a pivotal moment that threatened to derail the fragile truce. Tasha, fueled by her vision for a better future, stood firm against his proposition. "Razor, we can't build a future on the backs of our neighbors. The drug trade brings violence and fear, and that's not what this community deserves," she insisted, her voice steady but urgent
Razor, however, was unyielding. "You think your ideals can change the world. I'm in the real world, Tasha. Families are hungry. They want power and respect—what I can provide. You can't just erase the reality of survival."
Tasha's frustration mounted as she countered, "Meaningful change requires us to move away from illegal activities. We can create jobs and invest in our youth through legitimate means."
The tension in the room escalated, with Razor's gang members watching closely. Father Gregory attempted to mediate, sensing the critical impasse. "Perhaps there's a middle ground," he suggested, but Tasha was quick to interject.
"There is no middle ground when you're advocating for further destruction. I will not support a criminal approach to community development," she asserted. "We can uplift the community without violence."
Razor's demeanor softened slightly as he glanced around the room, noticing the murmurs of agreement with Tasha's vision. Yet he remained hesitant to concede control. "You can't just ask me to sacrifice everything without a viable alternative. Show me how your way will work, then we can talk."
Tasha took a deep breath, knowing this was a pivotal moment. "Let's invest in youth programs, job training, and small business grants. Work together to uplift the community without violence. I'll bring legitimate businesses in, and you can help steer that profit into community gains."
Razor stared at her, weighing his options. For so long, he had ruled through fear, convinced it was the only way. But now he faced a community unwilling to accept his old methods. "At the very least, I'll consider your proposal, Tasha," he finally said, his voice low but steady. "But if this doesn't strengthen my position, there will be consequences."
Tasha understood the fragility of this moment, but it was a step—a precarious but crucial step towards a newfound possibility for coexistence built on mutual benefit instead of mutual destruction. The fight for peace was far from over, and the battle lines continued to shift as they each sought to define their legacies amidst turbulent change.
Next sub-event:A betrayal by one of Razor's gang members forces him to reconsider his approach, realizing that his violent methods are leading to his downfall." 
\\ \\
\end{longtable}
